# Supplementary material for: Filter Functions for Quantum Processes under Correlated Noise
Source: arXiv:2103.02385 ancillary file (2021-10-25)
Supplement: Supplementary file 1 [file supplement.pdf]

# Supplemental Materials for Filter Functions for Quantum Processes under Correlated Noise

Pascal Cerfontaine,* Tobias Hangleiter, and Hendrik Bluhm
*JARA-FIT Institute for Quantum Information, Forschungszentrum Jülich GmbH and RWTH Aachen University, 52074 Aachen, Germany*

## I. DERIVING QUANTITIES FROM THE ERROR PROCESS $\tilde{\mathcal{U}}$

In this supplement we give a brief overview of scalar quantities that can be extracted from the quantum process $\mathcal{U} \equiv \mathcal{Q} \circ \tilde{\mathcal{U}}$, where $\tilde{\mathcal{U}}$ is the deviation from the ideal process $\mathcal{Q}$ due to noise given approximately by Eq. (4) of the main text. The ideal process is given simply by the unitary evolution after time $\tau$ of a gate operation, $\mathcal{Q}(\rho) = Q\rho Q^\dagger$ with $Q \equiv U_\mathrm{c}(\tau)$. To compute the quantities, one thus needs to obtain $\mathcal{Q}$ as well as $\tilde{\mathcal{U}}$ as described in the main text, and apply the prescriptions we detail below.

The average gate fidelity $\mathcal{F}$ was already discussed in the main text. Leakage can be computed following the definition given by Wood and Gambetta [1], who define leakage from one subspace of a composite Hilbert space $\mathscr{H} = \mathscr{H}_1 \oplus \mathscr{H}_2$ into another in terms of the projectors $\Pi_{1,2}$ onto the respective subspaces as follows:

$$L(\mathcal{U}) := \frac{1}{d_1} \operatorname{tr}(\Pi_2 \mathcal{U}(\Pi_1)) \tag{1}$$

where $d_{1,2}$ is the dimension of the subspaces.

The diamond distance to the identity gives the worst-case error of a gate implementation by maximizing the trace distance of the process to the identity, applied to the system part ($\mathscr{H}$) of a density operator on the Hilbert space extended by any ancilliary Hilbert space $\mathscr{H}'$, both over the ancilliary spaces $\mathscr{H}'$ and the density operators $\rho$ of the composite space. Mathematically, it is defined by [2]

$$d_\diamond(\tilde{\mathcal{U}}, \mathbb{1}) := \frac{1}{2}\|\tilde{\mathcal{U}} - \mathbb{1}\|_\diamond \tag{2}$$

with the diamond norm

$$\|\mathcal{U}\|_\diamond := \sup_{\mathscr{H}'} \sup_{\rho \in \mathrm{dens}(\mathscr{H} \otimes \mathscr{H}')} \|\mathcal{U} \otimes \mathbb{1}(\rho)\|_\mathrm{tr} \tag{3}$$

and the trace norm $\|A\|_\mathrm{tr} = \operatorname{tr}\sqrt{A^\dagger A}$. Thus, by numerically optimizing the suprema in Eq. (2) over the set of density operators $\mathrm{dens}(\mathscr{H} \otimes \mathscr{H}')$ and ancilliary Hilbert spaces $\mathscr{H}'$, it is possible to obtain an estimate of the diamond distance from the error process $\tilde{\mathcal{U}}$ derived in the main text.

* pascal.cerfontaine@rwth-aachen.de

Lastly, measurement probabilities can be extracted from Born's rule, which gives the probability of measuring an outcome $i$ associated with a POVM $\{E_i\}_i$ for a system prepared in the state $\rho$ and evolved under $\mathcal{U}$ as

$$p_i(\mathcal{U}, \rho) := \operatorname{tr}(E_i \mathcal{U}(\rho)). \tag{4}$$

Since $\mathcal{U}$ already contains the noise-averaged evolution, $p_i(\mathcal{U}, \rho)$ represents the probability that is expected to be observed after repeated measurements in the lab.

## II. QFT CONTROL AND NOISE MODEL

We assemble the quantum Fourier transform (QFT) circuit discussed in the main text from a minimal gate set consisting of three atomic gates, $\mathbb{G} = \{\mathrm{X}_i(\pi/2), \mathrm{Y}_i(\pi/2), \mathrm{CR}_{ij}(\pi/2^3)\}$ on or between qubits $i$ and $j$. We consider a simple model involving four single-spin qubits with in-phase (I) and quadrature (Q) single-qubit control and nearest neighbor exchange coupling so that the control Hamiltonian reads

$$H_\mathrm{c}(t) = \sum_{\langle i,j\rangle} I_i(t)\sigma_x^{(i)} + Q_i(t)\sigma_y^{(i)} + J_{ij}(t)\sigma_z^{(i)} \otimes \sigma_z^{(j)} \tag{5}$$

where $\sigma_\alpha^{(i)}$ is the trivial extension of the Pauli matrix $\sigma_\alpha$ of qubit $i$ to the full tensor product Hilbert space. For simplicity, we assume periodic boundary conditions so that qubits 1 and 4 are nearest neighbors as well. Similarly, we define the noise Hamiltonian as

$$H_\mathrm{n}(t) = \sum_{\langle i,j\rangle} b_I(t)\sigma_x^{(i)} + b_Q(t)\sigma_y^{(i)} + b_J(t)\sigma_z^{(i)} \otimes \sigma_z^{(j)} \tag{6}$$

with the noise fields $b_\alpha(t)$ for $\alpha \in \{I, Q, J\}$.

Using the QuTiP [3] implementation of GRAPE [4], we obtain the gate set $\mathbb{G}$. We compute the correlation filter functions (CFFs) as well as the correlation infidelities shown in the main text using the `filter_functions` software package [5], employing an efficient scheme based on the concatenation property (Eq. (10) of the main text) [6] . Figure S1 shows the quantum circuit diagram of the QFT algorithm with optional echo $\mathrm{X}(\pi)$-gates on qubit 4.

## III. VALIDATION OF QFT FIDELITIES

In this section, we perform Lindblad master equation and Monte Carlo simulations to verify the fidelities predicted for the QFT circuit in the main text. We focus

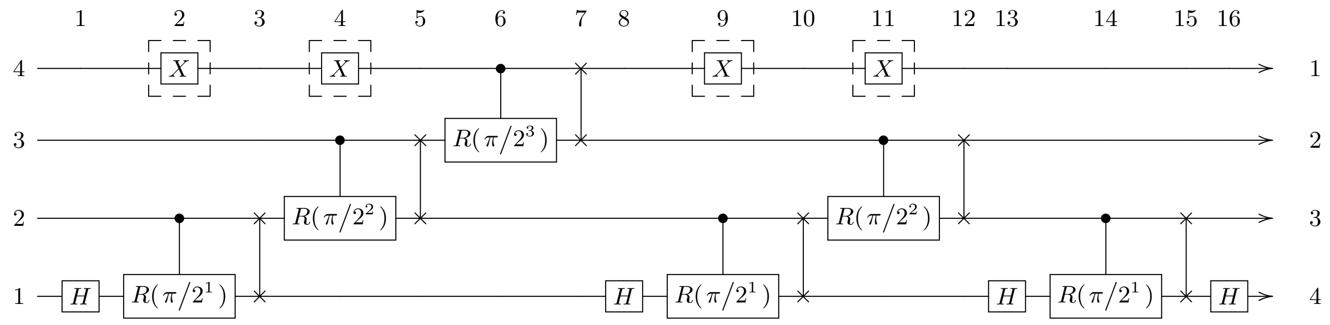

Figure S1. Quantum circuit diagram for a QFT circuit on four qubits with optional NOT gates implementing two consecutive Hahn echoes on qubit 4 which do not alter the computation. Numbers in the top row indicate the gate position $g$ in the circuit.

on noise exclusively on the third qubit, entering through the noise operator $B_\alpha \equiv \sigma_y^{(3)}$.

To validate the fidelity for white noise, we use a Lindblad master equation [7, 8] in superoperator form. We represent linear maps $\mathcal{A} : \rho \to \mathcal{A}(\rho)$ by matrices in the Pauli transfer matrix representation as (see Ref. 6 for more details)

$$\mathcal{A}_{ij} \coloneqq \mathrm{tr}(\sigma_i \mathcal{A}(\sigma_j)) \tag{7}$$

and operators as column vectors (i.e. generalized Bloch vectors) as

$$\rho_i \coloneqq \mathrm{tr}(\sigma_i \rho), \tag{8}$$

allowing us to write the Lindblad equation

$$\frac{\mathrm{d}}{\mathrm{d}t}\rho(t) = -\mathrm{i}[H(t), \rho(t)] + \sum_\alpha \gamma_\alpha \left( L_\alpha \rho(t) L_\alpha^\dagger - \frac{1}{2}\{L_\alpha^\dagger L_\alpha, \rho(t)\}\right) \tag{9}$$

as a linear differential equation in matrix form,

$$\frac{\mathrm{d}}{\mathrm{d}t}\rho_i(t) = \sum_j \left( -\mathrm{i}\mathcal{H}_{ij}(t) + \sum_\alpha \gamma_\alpha \mathcal{D}_{\alpha,ij}\right)\rho_j(t). \tag{10}$$

Here, $\mathcal{H}_{ij}(t) = \mathrm{tr}(\sigma_i[H(t), \sigma_j])$ and $\mathcal{D}_{\alpha,ij} = \mathrm{tr}\big(\sigma_i L_\alpha \sigma_j L_\alpha^\dagger - \frac{1}{2}\sigma_i\{L_\alpha^\dagger L_\alpha, \sigma_j\}\big)$. By setting $L_\alpha \equiv \sigma_y^{(3)}$ as well as $\gamma_\alpha \equiv S_0/2$ with $S_0$ the amplitude of the one-sided noise power spectral density (PSD) so that $S(\omega) = S_0$, we can compare the fidelity obtained from the filter functions to that from the explicit simulation of Eq. (10). The latter is computed as $\mathcal{F}_{\mathrm{avg}} = \mathrm{tr}\big(\mathcal{Q}^\dagger \mathcal{U}\big)/d^2$, where $\mathcal{Q}$ is the superpropagator due to the Hamiltonian evolution alone (i.e. the ideal evolution without noise).

For the Monte Carlo simulation, we explicitly generate time traces of $b_Q(t)$ (c.f. Eq. (6)) by drawing pseudo-random variables from a distribution whose PSD is $S(f) = S_0/f$. To do this, we draw complex, normally distributed samples in frequency space (i.e. white noise), scale it with the square root of the PSD, and finally perform the inverse Fourier transform. We choose an oversampling factor of 16, so that the time discretization of the simulation is $\Delta t_{\mathrm{MC}} = \Delta t/16 = 62.5\,\mathrm{ps}$ ($\Delta t = 1\,\mathrm{ns}$ is the time step of the pulses used in the FF simulation), leading to a highest resolvable frequency of $f_{\max} = 16\,\mathrm{GHz}$. Conversely, we increase the frequency resolution by sampling a time trace longer by a given factor, giving frequencies below $f_{\min}$ (16 kHz for pink, 0 Hz for white noise) weight zero, and truncating it to the number of time steps in the algorithm times the oversampling factor. This yields a time trace with frequencies $f \in [f_{\min}, f_{\max}]$ and a given resolution (we choose $\Delta f = 1.6\,\mathrm{kHz}$). For reference, we show the fidelity filter functions for the circuit with and without echo pulses in this frequency band in Fig. S2.

We then proceed to diagonalize the Hamiltonian $H(t) = H_c(t) + H_n(t)$ and compute the propagator for one noise realization as

$$U(t) = \prod_g V^{(g)} \exp\{-\mathrm{i}\Omega^{(g)}\Delta t_{\mathrm{MC}}\} V^{(g)\dagger}, \tag{11}$$

where $V^{(g)}$ is the unitary matrix of eigenvectors of $H(t)$ during time segment $g$ and $\Omega^{(g)}$ the diagonal matrix of eigenvalues. Finally, we obtain an estimate for the average gate fidelity $\mathcal{F}_{\mathrm{avg}}$ from the entanglement fidelity $\mathcal{F}_{\mathrm{e}}$ as

$$\langle \mathcal{F}_{\mathrm{avg}} \rangle = \left\langle \frac{d\mathcal{F}_{\mathrm{e}} + 1}{d+1} \right\rangle = \left\langle \frac{\big|\mathrm{tr}\big(Q^\dagger U(\tau)\big)\big|^2 + d}{d(d+1)} \right\rangle. \tag{12}$$

Here, $Q \equiv U_{\mathrm{c}}(t = \tau)$ is the noise-free propagator at time $\tau$ of completion of the circuit and $\langle\cdot\rangle$ denotes the ensemble average over $N$ Monte Carlo realizations of Eq. (11), i.e. $\langle A \rangle = \frac{1}{N}\sum_{i=1}^N A_i$. The standard error of the mean can be obtained as $\sigma_{\langle \mathcal{F}_{\mathrm{avg}}\rangle} = \sigma_{\mathcal{F}_{\mathrm{avg}}}/\sqrt{N}$ with $\sigma_{\mathcal{F}_{\mathrm{avg}}}$ the standard deviation over the Monte Carlo traces.

Table S1 compares the infidelities $\mathcal{I} = 1 - \mathcal{F}$ from Lindblad and Monte Carlo simulations to the filter function predictions following Eq. (11) of the main text. Note that the precise value of the filter function result depends quite sensitively on the frequency sampling due to the sharp peaks in the gigahertz range (Fig. S2). As the table shows, both the Lindblad and the Monte Carlo calculations agree well with the predictions made by our filter function formalism.

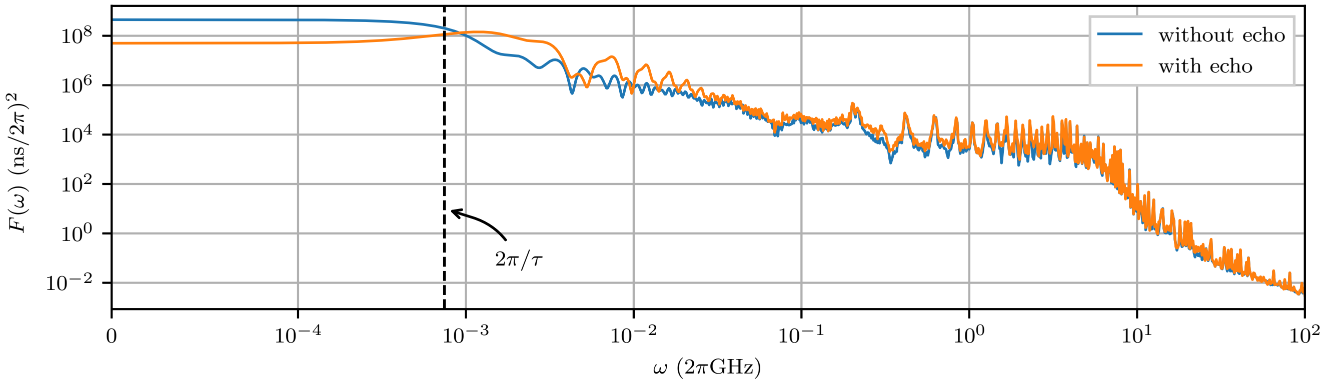


Figure S2. Filter functions for noise operator $\sigma_y^{(4)}$ for the QFT circuit without (blue) and with (orange) additional echo pulses. Introducing the echoes shifts spectral weight towards higher frequencies, reducing the DC level of the filter function by two orders of magnitude and thus leading to an improved fidelity for $1/f$ noise.

Table S1. Infidelities $\mathcal{I}_{\text{avg}} = 1 - \mathcal{F}_{\text{avg}}$ of the QFT circuit due to noise on $\sigma_y^{(3)}$. Monte Carlo values are given with the standard error of the mean for $N = 1008$. We included frequencies in the range of $\omega \in [0, 100]\,2\pi\text{GHz}$ for white noise, and $\omega \in [100\,2\pi\text{kHz}, 100\,2\pi\text{GHz}]$ for pink noise. Prefactors in the power law $S(\omega) = A\omega^\alpha$ are $2 \times 10^{-6}\,2\pi\text{GHz}$ and $1 \times 10^{-9}\,2\pi\text{GHz}^2$, respectively.

| Method | White noise | | $1/f$ noise | |
|---|---|---|---|---|
| | Without echo | With echo | Without echo | With echo |
| Lindblad | $8.38 \times 10^{-3}$ | $8.38 \times 10^{-3}$ | — | — |
| Monte Carlo | $(8.22 \pm 0.24) \times 10^{-3}$ | $(8.34 \pm 0.23) \times 10^{-3}$ | $(8.53 \pm 0.28) \times 10^{-3}$ | $(2.84 \pm 0.10) \times 10^{-3}$ |
| Filter functions | $8.34 \times 10^{-3}$ | $8.40 \times 10^{-3}$ | $8.34 \times 10^{-3}$ | $3.02 \times 10^{-3}$ |


[1] C. J. Wood and J. M. Gambetta, Phys. Rev. A **97**, 032306 (2018).

[2] Y. R. Sanders, J. J. Wallman, and B. C. Sanders, New Journal of Physics **18**, 012002 (2015).

[3] J. Johansson, P. Nation, and F. Nori, Computer Physics Communications **184**, 1234 (2013).

[4] T. Schulte-Herbrüggen, A. Spörl, N. Khaneja, and S. J. Glaser, Phys. Rev. A **72**, 042331 (2005).

[5] T. Hangleiter, I. N. M. Le, and J. D. Teske, "filter_functions: A package for efficient numerical calculation of generalized filter functions to describe the effect of noise on quantum gate operations," (2021), available at `https://github.com/qutech/filter_functions/`.

[6] T. Hangleiter, P. Cerfontaine, and H. Bluhm, "Filter function formalism and software package to compute quantum processes of gate sequences for classical non-markovian noise," [Reference inserted by publisher].

[7] G. Lindblad, Communications in Mathematical Physics **48**, 119 (1976).

[8] V. Gorini, A. Kossakowski, and E. C. G. Sudarshan, Journal of Mathematical Physics **17**, 821 (1976).
